# Supplementary material for: RF Helicon Plasma Thruster for an Atmosphere-Breathing Electric Propulsion System (ABEP)
Source: arXiv:2607.02635 source file (2026-07-02)
Supplement: Supplementary file 1 [file appendixA.tex]

%\subsubsection{Class E-Amplifier}
The RF generator used for IPT is based on a Class E-Amplifier. These devices are all derived from a basic RLC circuit. A basic switching amplifier is shown within Fig.~\ref{fig:simpleswitch-IV}. The switch is considered ideal so to be either completely open or completely closed, and the change between the two states is instantaneous, see the $I$ and $V$ diagrams in Fig.~\ref{fig:simpleswitch-IV}.\begin{figure}[hp]
	\centering
	\includegraphics[width=6cm]{bilder/RF/rf-switch-amplifier}
	\qquad
	\includegraphics[width=6cm]{bilder/RF/rf-switch-amplifier-IV}
	\caption{Basic RF switching amplifier (left),and its $I$ and $V$ output profiles,~\cite{9781596930186}.}
	\label{fig:simpleswitch-IV}
\end{figure}

The E-class differs from the standard amplifier of Fig.~\ref{fig:simpleswitch-IV} as the ideal switch has a capacitor in parallel that shunts it~\cite{9781596930186}. The DC voltage $V_{DC}$ is supplied through a high-reactance choke that does not support any current variation of one RF cycle. The rest of the circuit is a resonant circuit that contains also the final RF load resistor, usually of \SI{50}{\ohm}. The assumptions are that the current in the RLC branch, $I_{rf}\sin{\omega t}=I_{rf}\sin{\theta}$, is sinusoidal, and that the switch opening and closing timing can be arbitrarily selected. The current flowing through the switch is $i(\theta)=I_{dc}+I_{rf}\sin{\theta}$. The main important feature is that if the switch is closed, $i_{sw}(\theta)$ flows completely through the switch, while if the switch is opened, it will flow completely through the shunt capacitor $C_P$. The current flowing through $C_P$ is an offset for the sinusoidal current. As in Fig.~\ref{fig:Eswitch-IV}, as the switch triggers, the current goes from switch to capacitor. The closing of the switch happens exactly as $i_{rf}(\theta)$ passes by $0$. Finally the E-class amplifier highlights are shown in the bullet list below.\begin{itemize}
	\item Conversion efficiency of DC to RF is $100\%$, as at no time current and voltage are both zero;
	\item The only dissipative component of the circuit is the load resistor and it is visible only at the switching frequency, the energy is dissipated on it only at that frequency;
	\item The waveform of the voltage is non-sinusoidal and axially asymmetric, the mean DC level will be lower than $V_{peak}/2$.
\end{itemize}
\begin{figure}[h]
	\centering
	\includegraphics[width=7cm]{bilder/RF/rf-switch-amplifierE}
	\caption{Class E amplifier scheme~\cite{9781596930186}.}
	\label{fig:Eswitch-IV}
	\includegraphics[width=6.5cm]{bilder/RF/rf-switch-amplifierE-IV}
	\qquad
	\includegraphics[width=6.5cm]{bilder/RF/rf-switch-amplifierE-IV-b}
	\caption{Class E amplifier, $i(\theta),~i_{sw}(\theta),~i_{c}(\theta),~v_c({\theta})$ profiles,~\cite{9781596930186}.}
	\label{fig:Eswitch-IV-b}
\end{figure}
Finally, the main advantage of an E-class amplifier its is high efficiency, that also leads to low heat generation, albeit very high RF voltage peaks.
